# Supplementary material for: Information retrieval and eigenstates coalescence in a non-Hermitian quantum system with anti-$\mathcal{PT}$ symmetry
Source: arXiv:2107.12635 source file (2021-07-27)
Supplement: Supplementary file 1 [file supplementary.pdf]

# Supplemental Material for "Information retrieval and eigenstates coalescence in a non-Hermitian quantum system with anti-$\mathcal{PT}$ symmetry"

Liangyu Ding,[1] Kaiye Shi,[1] Yuxin Wang,[1] Qiuxin Zhang,[1] Chenhao Zhu,[1] Ludan Zhang,[1] Jiaqi Yi,[1] Shuaining Zhang,[1, 2, 3] Xiang Zhang,[1, 2, 3, *] and Wei Zhang[1, 2, 3, †]

[1]*Department of Physics, Renmin University of China, Beijing 100872, China*
[2]*Beijing Academy of Quantum Information Sciences, Beijing 100193, China*
[3]*Beijing Key Laboratory of Opto-electronic Functional Materials and Micro-nano Devices, Renmin University of China, Beijing 100872,China*

## EXPERIMENTAL SYSTEM AND ERROR ANALYSIS

The ion is trapped in a 4-rod trap and cooled by a beam of 369.5nm containing $\sigma_+$, $\sigma_-$ and $\pi$ polarizations with a re-pumping beam of 935nm which is used to re-pump the leakage on the other metastable state and completes a stable Doppler cooling scheme as shown in Fig. 1(b) of the main text. The beam of 369.5nm with different energy shift can also be used for detecting the final state and pumping the state to the ground state.

In our experiment, we demonstrate variation of the observables with respect to time-dependent coupling strength $J(t)$, detuning $\delta(t)$ and dissipation rate $\Gamma(t)$. The inter-spin coupling is driven by a microwave horn antenna transmitting signal of frequency $\omega_{\rm HF} = 12.642812118466$ GHz $+ \Delta_B$, which is the energy gap between $|\uparrow\rangle$ and $|\downarrow\rangle$ states. Here, $\Delta_B = 310.8B^2$ Hz and $B$ is the magnetic field around the ion in the unit of Gauss (Gs). This signal is generated by mixing a 12.4 GHz stable signal source with a 1.2 GS/s (Giga samples per second) arbitrary waveform generator (AWG). The coupling strength $J$ is controlled by the amplitude of the microwave and measured by fitting the Rabi frequency.

In our experiment, we periodically vary the parameters $J_i$ and $\Gamma_2$ in forms of symmetric square function as shown in Fig. 1(c) of the main text. The maximal amplitude of $J(t)$ is 0.206 MHz. The detuning $\delta$ is set by the AWG as well, ranging from -0.16 MHz to 0.16 MHz. We use permanent magnets and Helmholtz coils to create a magnetic field around 10 Gs. As a result, there is a 14 MHz Zeeman splitting between $|\uparrow\rangle \equiv |F = 1, m_F = 0\rangle$ and $|F = 1, m_F = \pm 1\rangle$ of the $^2S_{1/2}$ manifold. Thus, the detuning applied in our experiment is nearly two orders of magnitude smaller than the Zeeman splitting. The dissipation of $|\uparrow\rangle$ state is generated by a 396.5 nm beam as shown in Fig. 1(a) of the main text. The beam has passed through a linear polarizer and contains only $\pi$-polarization components parallel to the magnetic field, such that the other Zeeman levels in the $\left|^2S_{1/2}, F = 1\right\rangle$ manifold will not be excited owing to selection rules. The lifetime of $\left|^2P_{1/2}, F = 0\right\rangle$ state is short enough comparing to the beam strength and the state will spontaneously decay to $\left|^2S_{1/2}, F = 1\right\rangle$ states with equal probabilities. It has been demonstrated that the Hamiltonian of this quantum process can be written as $-i\Gamma |\uparrow\rangle\langle\uparrow|$, so that we can obtain the effective dissipation rate $\Gamma$ from a fitting of exponential decay of spin population [1].

The system is relatively stable during one round of experiment so that we are mainly concerned with the quantum projection noise, which can be suppressed by increasing the number of measurements. We repeat each measurement 1,000 times to get the expectation value. The statistical errors are estimated by one standard deviation with the standard error propagation method of the measured observables. The fluctuation of control parameters is the dominant error source in our experiment. The relative error is 1.4% for the coupling strength $J$ and 5% for the dissipation rate $\Gamma$ measured by repeatedly conduct the fitting sequence for 20 rounds. One may notice that in Figs. 2(c), 3, and 4 in the main text, the error bars of some data points are fairly significant. This is because the expressions into which the measured data are substituted behave sensitively on input variables in certain regimes.

## EFFECTIVE FLOQUET HAMILTONIAN WITH ANTI-$\mathcal{PT}$ SYMMETRY

We divide the cycle $T$ of the periodic driving into three segments, i.e., $T_1$, $T_2$ and $T_3$, with corresponding Hamiltonians $\hat{H}_1$, $\hat{H}_2$ and $\hat{H}_3$, respectively. The instantaneous Hamiltonian takes the form

$$\hat{H}_i(t) = J_i(t) e^{-i\phi_i(t)\hat{\sigma}_z} \hat{\sigma}_x - 2i\Gamma_i(t) |\uparrow\rangle\langle\uparrow| , \tag{1}$$

where $J_i$, $\Gamma_i$ and $\phi_i$ with $i = 1, 2, 3$ are time-dependent parameters. The effective Floquet Hamiltonian is $\hat{H}_F = i\log\left(\hat{U}_T\right)/T$, where $\hat{U}_T = e^{-i\hat{H}_3 T_3} e^{-i\hat{H}_2 T_2} e^{-i\hat{H}_1 T_1}$. We set $\phi_1 = -\pi/2$, $\phi_2 = 0$, $\phi_3 = \pi/2$, and $J_1 T_1 = J_3 T_3 = \pi/4$. Thus, the driving period is $T = \pi/4J_1 + \pi/4J_2 + T_2$.

For a Hamiltonian in the form $\hat{H} = \boldsymbol{h}\cdot\hat{\boldsymbol{\sigma}}$ where $\hat{\boldsymbol{\sigma}}$ is the Pauli matrix vector, the Euler's formula of the Pauli matrix is

$$e^{-i\boldsymbol{h}\cdot\hat{\boldsymbol{\sigma}}t} = \cos(\varepsilon t) - i\sin(\varepsilon t)\boldsymbol{h}\cdot\hat{\boldsymbol{\sigma}}/\sqrt{\boldsymbol{h}\cdot\boldsymbol{h}}. \tag{2}$$

where $\varepsilon$ is the deterministic of $\boldsymbol{h}$. Use this identity, we have the following expression for the evolution operator

$$\begin{aligned}
\hat{U}_T &= \frac{e^{-\Gamma T_2}}{2}(1 - i\hat{\sigma}_y)\left(\cos T_2\varepsilon - i\frac{\hat{H}_{\mathcal{PT}}}{\varepsilon}\sin T_2\varepsilon\right)(1 + i\hat{\sigma}_y) \\
&= e^{-\Gamma T_2}\left\{\cos\left[\left(\frac{T_2}{T}\varepsilon\right)T\right] - \frac{T_2}{T}\frac{i\hat{H}_{\mathcal{PT}}\hat{\sigma}_y - i\hat{\sigma}_y\hat{H}_{\mathcal{PT}}}{2\frac{T_2}{T}\varepsilon} i\sin\left[\left(\frac{T_2}{T}\varepsilon\right)T\right]\right\} \\
&\equiv e^{-\Gamma T_2}\hat{U} \\
&\equiv e^{-i\hat{H}_F T},
\end{aligned} \tag{3}$$

where $\hat{U}$ is defined as the content in the bracket. Using the Euler's formula again, we obtain the effective Hamiltonian,

$$\begin{aligned}
\hat{H}_F &= \frac{i}{T}\log\left(e^{-\Gamma T_2}\hat{U}\right) \\
&= \frac{i}{T}\left[\log\left(\hat{U}\right) + \log\left(e^{-\Gamma T_2}\right)\right] \\
&= i\frac{\hat{H}_{\mathcal{PT}}T_2}{2T}\hat{\sigma}_y - i\hat{\sigma}_y\frac{\hat{H}_{\mathcal{PT}}T_2}{2T} - i\Gamma\frac{T_2}{T}\hat{\mathcal{I}} \\
&= \frac{T_2}{T}\left(-J\hat{\sigma}_z - i\Gamma\hat{\sigma}_x - i\Gamma\hat{\mathcal{I}}\right).
\end{aligned} \tag{4}$$

It's straightforward to verify that $\hat{\mathcal{P}}\hat{\mathcal{T}}\hat{H}_F\hat{\mathcal{P}}\hat{\mathcal{T}} = -\hat{H}_F$, where $\hat{\mathcal{P}} = \hat{\sigma}_x$ and $\hat{\mathcal{T}}$ represents complex conjugate. Therefore, we can directly implement a Floquet Hamiltonian with anti-$\mathcal{PT}$ symmetry. Its eigenvalues are $E_\pm = \alpha(-i\Gamma \pm \varepsilon)$ and the corresponding eigenvectors is $|\varphi_\pm\rangle$, where $\alpha = T_2/T$. In our experiment, we set $0.05 \le \alpha \le 0.72$.

## DETECTION OF EIGENSTATES VIA DENSITY MATRIX EVOLUTION

In the anti-$\mathcal{PT}$ symmetry broken phase, the time evolution of an initial state $|\psi\rangle = c_+|\varphi_+\rangle + c_-|\varphi_-\rangle$ can be written as

$$\begin{aligned}
|\psi, t\rangle &= c_+ e^{-iE_+ t}|\varphi_+\rangle + c_- e^{-iE_- t}|\varphi_-\rangle \\
&= e^{-iE_+ t}\left[c_+|\varphi_+\rangle + c_- e^{-i(E_- E_+)t}|\varphi_-\rangle\right] \\
&= e^{-iE_+ t}\left[c_+|\varphi_+\rangle + c_- e^{i\alpha\varepsilon t}|\varphi_-\rangle\right],
\end{aligned} \tag{5}$$

where $c_\pm$ are the corresponding projection on thee two eigenstates. In the last line of the expression above, we use the property that when the anti-$\mathcal{PT}$ symmetry is broken with , the two eigenvalues $E_\pm$ acquire a same imaginary part and opposite real parts, such that $E_- E_+ = -\alpha\varepsilon = -i\alpha|\varepsilon|$. Thus, we obtain

$$|\psi, t\rangle = e^{-iE_+ t}\left[c_+|\varphi_+\rangle + c_- e^{-\alpha|\varepsilon|t}|\varphi_-\rangle\right]. \tag{6}$$

In the long time limit $t \to +\infty$, we have $e^{-\alpha|\varepsilon|t} \to 0$, and $|\psi, +\infty\rangle = e^{-iE_+ t}c_+|\varphi_+\rangle$. Thus,

$$\bar{\rho}(+\infty) = \frac{|\psi, +\infty\rangle\langle\psi, +\infty|}{|\langle\psi, +\infty|\,\psi, +\infty\rangle|^2} = |\varphi_+\rangle\langle\varphi_+|. \tag{7}$$

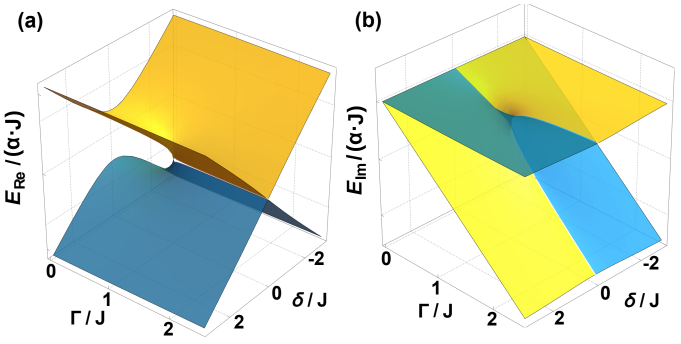


Figure S1. (a) The real and (b) imaginary parts of the two eigenvalue of the Hamiltonian $\hat{H}_F^\delta$, as functions of $\delta/J$ and $\Gamma/J$. The orange and blue sheets denote the results correspond to the $E_+^\delta$ and $E_-^\delta$ branches, respectively.

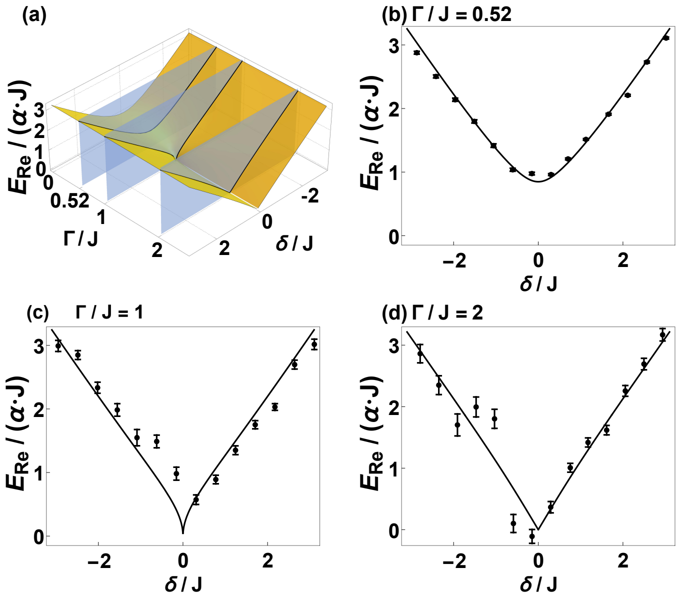


Figure S2. (a) The real part of the $E_+$ brach eigenvalue in the parameter space spanned by $\delta/J$ and $\Gamma/J$ (orange surfaces). The three semi-lucent cross sections (gray surfaces) with interaction lines denote a fixed value of $\Gamma/J = 0.52$, 1, and 2, respectively. (b-d) The numerical results (solid lines) are compared with experimental data (points with error bars).

In order to prepare $|\varphi_-\rangle$, we reverse the driving sequence of Hamiltonian, so that the evolution is governed by $\hat{U}_{T,r} = e^{-i\hat{H}_1 T_1} e^{-i\hat{H}_2 T_2} e^{-i\hat{H}_3 T_3}$. The effective Hamiltonian of the reversed evolution, $\hat{H}_{F,r}$, has the same eigensrtates with $\hat{H}_F$ because $\hat{H}_{F,r} = -\hat{H}_F - 2i\Gamma\hat{\mathcal{I}}$. In fact, we can obtain $\hat{H}_{F,r}\,|\varphi_\pm\rangle = (-E_\pm - 2i\Gamma)\,|\varphi_\pm\rangle = E_\pm^r\,|\varphi_\pm\rangle$. Since $\mathrm{Im}(E_+^r) < \mathrm{Im}(E_-^r)$, after the same analysis as above, we can get

$$\bar{\tilde{\rho}}(+\infty) = |\varphi_-\rangle\langle\varphi_-|\,. \tag{8}$$

## TOPOLOGICAL CHARACTERISTICS AROUND EP

To reveal the topological characteristics of the eigenvalue sheets around EP, we impose a detuning $\delta$ of the inter-spin coupling, such that the middle segment of a driving period is $\hat{H}_2^\delta = \delta\hat{\sigma}_z + \hat{H}_2$. The effective Floquet Hamiltonian then becomes

$$\hat{H}_F^\delta = \alpha[(\delta - i\Gamma)\hat{\sigma}_x - J\hat{\sigma}_z - i\Gamma\hat{\mathcal{I}}], \tag{9}$$

and the eigenvalues are $E_\pm^\delta = \alpha(-i\Gamma \pm \varepsilon^\delta)$, where $\varepsilon^\delta = \sqrt{J^2 + (\delta - i\Gamma)^2}$. The dimensionless parameters $\delta/J$ and $\Gamma/J$ span the parameter space in which the eigenvalues form Riemann surfaces.

As shown in Fig. S1, the two intersecting Riemann surfaces wrap around the EP, leading to a second-order branch-point singularity [2], which is responsible to the square root response of energy splitting to the perturbation [3, 4]. This non-trivial topological structure of EP does not exist around a DP, where a double-cone topological structure appears with linear energy splitting and no branch-point singularity [2, 3]. Thus, the enhancement of sensitivity is a characteristic feature of EP, which does not present for a DP [5, 6].

For a system not exactly at EP, the evolution of an initial state $\left|\psi^{\delta}, t=0\right\rangle = c_{+}^{\delta}\left|\varphi_{+}^{\delta}\right\rangle + c_{-}^{\delta}\left|\varphi_{-}^{\delta}\right\rangle$ can be expressed as $\left|\psi^{\delta}, t\right\rangle = c_{+}^{\delta}e^{-iE_{+}^{\delta}t}\left|\varphi_{+}^{\delta}\right\rangle + c_{-}^{\delta}e^{-iE_{-}^{\delta}t}\left|\varphi_{-}^{\delta}\right\rangle$, where $\left|\varphi_{\pm}^{\delta}\right\rangle$ are the eigenvectors of Eq. (9). Thus, the population of $|\downarrow\rangle$ at time $t$ is

$$\left|\langle\downarrow|\psi^{\delta}, t\rangle\right|^{2} = \left|c_{+}^{\delta}e^{-iE_{+}^{\delta}t}\left\langle\downarrow|\varphi_{+}^{\delta}\right\rangle + c_{-}^{\delta}e^{-iE_{-}^{\delta}t}\left\langle\downarrow|\varphi_{-}^{\delta}\right\rangle\right|^{2}. \quad (10)$$

In the experiment, we choose the initial state as $\left|\psi^{\delta}, 0\right\rangle = |\downarrow\rangle$, such that Eq. (10) can be simplified as

$$\left|\langle\downarrow|\psi^{\delta}, t\rangle\right|^{2} = e^{-2\Gamma t}\left|\cos\left(\alpha\varepsilon^{\delta}t\right) - iJ\sin\left(\alpha\varepsilon^{\delta}t\right)/(\varepsilon^{\delta})\right|^{2}. \quad (11)$$

By fitting the experimental results with respect to the expression above, we can extract the deterministic $\varepsilon^{\delta}$ and the eigenvalues $E_{\pm}^{\delta} = \alpha(-i\Gamma \pm \varepsilon^{\delta})$. As an example, we show the experimental measurement of the real part of $E_{+}^{\delta}$ in Fig. S2, and the imaginary part in Fig. 5 of the main text.

* siang.zhang@ruc.edu.cn
† wzhangl@ruc.edu.cn

[1] L. Ding, K. Shi, Q. Zhang, D. Shen, X. Zhang, and W. Zhang, Experimental determination of $\mathcal{PT}$-symmetric exceptional points in a single trapped ion, Phys. Rev. Lett. **126**, 083604 (2021).
[2] Ş. K. Özdemir, S. Rotter, F. Nori, and L. Yang, Parity-time symmetry and exceptional points in photonics, Nat. Mater. **18**, 783 (2019).
[3] Y. Ashida, Z. Gong, and M. Ueda, Non-Hermitian physics, Adv. Phys. **69**, 249 (2020).
[4] W. D. Heiss, Chirality of wavefunctions for three coalescing levels, J. Phys. A Math. Theor. **41**, 244010 (2008).
[5] H. Hodaei, A. U. Hassan, S. Wittek, H. Garcia-Gracia, R. El-Ganainy, D. N. Christodoulides, and M. Khajavikhan, Enhanced sensitivity at higher-order exceptional points, Nature **548**, 187 (2017).
[6] L. Pan, S. Chen, and X. Cui, High-order exceptional points in ultracold bose gases, Phys. Rev. A **99**, 011601 (2019).
